# Supplementary material for: A Deeper Dive Into What Deep Spatiotemporal Networks Encode: Quantifying Static vs. Dynamic Information
Source: arXiv:2206.02846 source file (2022-06-06)
Supplement: Supplementary file 1 [file vos_supplementary.tex]

Supplementary materials adding all thresholds experiment in Figure~\ref{fig:vos_allthresholds} 

All thresholds:
\input{tex/graphs/vos_arch_indiv_allthresholds}

Fusion Layers:
\input{tex/graphs/vos_arch_indiv_fusionlayers}

%MATNet Variants:
%\input{tex/graphs/vos_arch_suppl}

All thresholds experiment on VOS datasets in Figure~\ref{fig:vos_allthresholds_dataset}.

\input{tex/graphs/vos_dataset_indiv_allthresholds}

evaluating on both DAVIS~\cite{Perazzi2016} and camouflaged moving objects dataset (MoCA)~\cite{lamdouar2020betrayed}. For MATNet results on MoCA we report it from~\cite{yang2021selfsupervised} as ``MATNet Original'', while MATNet~\cite{zhou2020motion} and RTNet~\cite{ren2021reciprocal} results on DAVIS are reported from their original works. We reproduce MATNet with an improved performance running with larger batch size=6. Then train for MATNet without boundary aware refinement modules. It is worth noting evaluating for our reproduce versions of MATNet ensures no horizontal flipping is used during inference unlike what the original MATNet was doing for fair comparison with RTNet. We select MoCA specifically for evaluation as it contains sequences where the objects' appearance is camouflaged with the surrounding background and in some sequences it is harder to segment based on static images solely. 

% MATNet No BAR: (0.672). SR at 0.5: (0.770), 0.6: (0.708), 0.7: (0.604), 0.8: (0.436), 0.9: (0.199),
% MATNet: Js: (0.678). SR at 0.5: (0.780), 0.6: (0.723), 0.7: (0.613), 0.8: (0.452), 0.9: (0.215),
% MATNet No BAR (no flipping in inference): Js: (0.651). SR at 0.5: (0.736), 0.6: (0.680), 0.7: (0.589), 0.8: (0.447), 0.9: (0.215),
% MATNet DAVIS Only: Js: (0.547). SR at 0.5: (0.599), 0.6: (0.535), 0.7: (0.440), 0.8: (0.310), 0.9: (0.134),
% MATNet (no flipping in inference): (0.669). SR at 0.5: (0.765), 0.6: (0.708), 0.7: (0.609), 0.8: (0.460), 0.9: (0.235),
% RTNet: Js: (0.607). SR at 0.5: (0.679), 0.6: (0.624), 0.7: (0.536), 0.8: (0.434), 0.9: (0.239),
% FusionSeg: Js: (0.423). SR at 0.5: (0.479), 0.6: (0.436), 0.7: (0.359), 0.8: (0.242), 0.9: (0.094),

\begin{table*}[t]
    \centering
\begin{tabular}{|l|c|ccccccc|}
\hline
\multirow{3}{*}{Method} & DAVIS & \multicolumn{7}{c|}{MoCA} \\ \cline{2-9} 
& \multirow{2}{*}{mIoU} & \multirow{2}{*}{mIoU} & \multicolumn{6}{c|}{Success Rate} \\
&  &  & $\tau=0.5$ & $\tau=0.6$ & $\tau=0.7$& $\tau=0.8$ &  $\tau=0.9$ &  $SR_{\text{Mean}}$\\ \hline
FusionSeg~\cite{jain2017fusionseg} Modified & 70.8 & 42.3 & 47.9 & 43.6 & 35.9 & 24.2 & 9.4 & 39.2\\
RTNet~\cite{ren2021reciprocal} & 85.6 & 60.7 & 67.9 & 62.4 & 53.6 & 43.4 & 23.9 & 50.2 \\
MATNet~\cite{zhou2020motion} Original & 82.4 & 64.2 & 71.2 & 67.0 & 59.9 & 49.2 & 24.6 & 54.4 \\
MATNet reproduced & - & 66.9 & 76.5 & 70.8 & 60.9 &46.0 & 23.5 & 55.5\\
MATNet No BAR & - & 65.1 & 73.6 & 68.0 & 58.9 & 44.7 & 21.5 &  53.3\\ \hline
\end{tabular}
    \caption{Caption}
    \label{tab:moca_vs_davis}
\end{table*}

\input{tex/graphs/vos_arch_jointtodynamic}

\begin{figure*}[t]
\centering
%\begin{subfigure}{.33\textwidth}
%    \includegraphics[width=\textwidth]{tex/images/vos_joint_encoding_neurons/fseg/raw_layer4,sensor_fusion.png}
%    \caption{}
%\end{subfigure}%
%\begin{subfigure}{.33\textwidth}
%    \includegraphics[width=\textwidth]{tex/images/vos_joint_encoding_neurons/matnet/raw_layer4,sensor_fusion.png}
%    \caption{}
%\end{subfigure}%
%\begin{subfigure}{.33\textwidth}
%    \includegraphics[width=\textwidth]{tex/images/vos_joint_encoding_neurons/rtnet/raw_layer4,sensor_fusion.png}
%    \caption{}
%\end{subfigure}%

\begin{subfigure}{.16\textwidth}
    \includegraphics[width=\textwidth]{tex/images/fusionseg/app_fseg.png}
    \caption{}
\end{subfigure}%
\begin{subfigure}{.16\textwidth}
    \includegraphics[width=\textwidth]{tex/images/fusionseg/mot_fseg.png}
    \caption{}
\end{subfigure}%
\begin{subfigure}{.16\textwidth}
    \includegraphics[width=\textwidth]{tex/images/matnet/app_matnet.png}
    \caption{}
\end{subfigure}%
\begin{subfigure}{.16\textwidth}
    \includegraphics[width=\textwidth]{tex/images/matnet/mot_matnet.png}
    \caption{}
\end{subfigure}%
\begin{subfigure}{.16\textwidth}
    \includegraphics[width=\textwidth]{tex/images/rtnet/app_rtnet.png}
    \caption{}
\end{subfigure}%
\begin{subfigure}{.16\textwidth}
    \includegraphics[width=\textwidth]{tex/images/rtnet/mot_rtnet.png}
    \caption{}
\end{subfigure}

    \caption{Individual Units Analysis Histograms in (a,b) FusionSeg~\cite{jain2017fusionseg} modified and (c,d) MATNet~\cite{zhou2020motion} respectively. It shows the histogram for static (a,c) and dynamic (b,d) factors for both models. }
    \label{fig:vos_indiviual_units}
\end{figure*}

performance improvement on MoCA w.r.t rest of models is confounding of both motion-to-appearance cross connections (push the model for higher specialized dynamic and static units) and training on additional Youtube-VOS dataset affects Joint/Dynamic relative percentage. Thus the best model we have evaluated on MoCA has higher number of static/dynamic specialized units without completely ignoring the jointly encoding units as happened in MATNet trained on DAVIS only.
